# Supplementary material for: Measurement of $CP$ violation in $B^0\rightarrow J/\psi K^0_\mathrm{S}$ and $B^0\rightarrow\psi(2S) K^0_\mathrm{S}$ decays
Source: arXiv:1709.03944 source file (2018-01-11)
Supplement: Supplementary file 2 [file supplementary-app.tex]

\clearpage

\section{Supplementary material for LHCb-PAPER-20XX-YYY}
\label{sec:Supplementary-App}

This appendix contains supplementary material that will posted
on the public cds record but will not appear in the paper.

Please leave the above sentence in your draft for first and 
second circulation and replace what follows by your actual supplementary material.
For more information about other types of supplementary material, see Section~\ref{sec:Supplementary}. Plots and tables that follow should be well described, either with captions or with additional explanatory text.

\begin{figure}[!htb]
  \begin{center}
    \includegraphics[scale=0.65,bb=50 300 580 700,clip=true]{Roger-plot}
    \vspace*{-1.0cm}
  \end{center}
  \caption{
    \small %captions should be a little bit smaller than main text
    Comparison of our result to those from other experiments.
    Note that the style of this figure differs slightly from that of Figure~\ref{fig:example}}
  \label{fig:roger}
\end{figure}

\clearpage
